# Supplementary material for: The Fisher-Rao geometry of CES distributions
Source: arXiv:2310.01032 source file (2023-10-02)
Supplement: Supplementary file 1 [file Appendix.tex]

\subsection{Proof of Theorem~\ref{thm:fisher_metric_ces}}
\label{appendix:proof_fim}

The Fisher Information Metric is obtained according to Theorem \ref{thm:smith_fim} as
\begin{equation}
\label{eq:proof_eq_thm3}
g^{fim}_{\boldsymbol{\Sigma}} \left(   \boldsymbol{\Omega},   \boldsymbol{\Omega} \right) = - \mathbb{E} \left[ ~ \left.  \frac{\text{d}^2}{\text{d}t^2} \mathcal{L} \left(  \{ \mathbf{z}_k \} | \boldsymbol{\Sigma} +  t \partial \boldsymbol{\Omega} , g\right) \right|_{t=0}~ \right]
.
\end{equation}
First, recall that the log-likelihood of the sample set is
\begin{equation}
\small
\mathcal{L}\left(  \{ \mathbf{z}_k \} | \boldsymbol{\Sigma},g \right)   = 
 \sum_{k=1}^K  \log \left(  g \left(  {\rm Tr} \left\{  \boldsymbol{\Sigma}^{-1} \mathbf{Z}_k  \right\} \right) \right)
 - K  \log |\boldsymbol{\Sigma}| 
 ,
\end{equation}
where $\mathbf{Z}_k = \mathbf{z}_k\mathbf{z}_k^H $.
We have the following Taylor expansions of order two around $\boldsymbol{\Sigma}$:
\begin{equation}
\footnotesize
\begin{aligned}
 \log | \boldsymbol{\Sigma}+  t\boldsymbol{\Omega} |  =
\log | \boldsymbol{\Sigma}  | 
+  {\rm Tr} \left\{   \boldsymbol{\Sigma}^{-1} t \boldsymbol{\Omega}  \right\} 
- \frac{1}{2} {\rm Tr } \left\{ \left( \boldsymbol{\Sigma}^{-1} t \boldsymbol{\Omega} \right)^2 \right\} + \ldots
\end{aligned}
\end{equation}
and
\begin{equation}
\footnotesize
\begin{aligned}
& \log \left(  g \left(   {\rm Tr} \left\{ \left( \boldsymbol{\Sigma} + t \boldsymbol{\Omega} \right)^{-1} \mathbf{Z}_k  \right\} \right)  \right) = 
 ~~
\log \left(  g \left(   {\rm Tr} \left\{  \boldsymbol{\Sigma}^{-1} \mathbf{Z}_k  \right\} \right)  \right) 
\\
&
~~~~~~~~~~~~~~~~
- {\rm Tr} \left\{ \boldsymbol{\Sigma}^{-1} t \boldsymbol{\Omega}  \boldsymbol{\Sigma}^{-1} \mathbf{Z}_k \right\}  \psi \left( {\rm Tr}\left\{  \boldsymbol{\Sigma}^{-1} \mathbf{Z}_k  \right\} \right) 
\\
&
~~~~~~~~~~~~~~~~
+ {\rm Tr} \left\{ \left( t \boldsymbol{\Omega} \boldsymbol{\Sigma}^{-1} \right)^2  \mathbf{Z}_k \boldsymbol{\Sigma}^{-1} \right\}    \psi \left( {\rm Tr}\left\{  \boldsymbol{\Sigma}^{-1} \mathbf{Z}_k  \right\} \right) 
\\
&
~~~~~~~~~~~~~~~~
+ \frac{1}{2}     {\rm Tr}^2\left\{ \boldsymbol{\Sigma}^{-1} t \boldsymbol{\Omega} \boldsymbol{\Sigma}^{-1} \mathbf{Z}_k \right\}
\psi' \left(   Tr \left\{  \boldsymbol{\Sigma}^{-1} \mathbf{Z}_k \right\} \right)
+ \ldots
\end{aligned}
\end{equation}
By removing the higher order terms we obtain
\begin{equation}
\label{eq:proof_taylor}
\footnotesize
\begin{aligned}
&
\left.  \frac{\text{d}^2}{\text{d}t^2} \mathcal{L} \left(  \{ \mathbf{z}_k \} | \boldsymbol{\Sigma} +  t  \boldsymbol{\Omega} \right) \right|_{t=0} = ~~
 K {\rm Tr} \left\{ \left(  \boldsymbol{\Omega}  \boldsymbol{\Sigma}^{-1} \right)^2 \right\}  
\\
&~~~~~~~~~~~~~
+ 2 \sum_{k=1}^K    
  {\rm Tr} \left\{ \left(   \boldsymbol{\Omega} \boldsymbol{\Sigma}^{-1} \right)^2  \mathbf{Z}_k \boldsymbol{\Sigma}^{-1} \right\}    \phi \left( Tr\left\{  \boldsymbol{\Sigma}^{-1} \mathbf{Z}_k  \right\} \right)   
\\
&~~~~~~~~~~~~~
+ \sum_{k=1}^K     {\rm Tr}^2\left\{ \boldsymbol{\Sigma}^{-1}   \boldsymbol{\Omega}  \boldsymbol{\Sigma}^{-1} \mathbf{Z}_k \right\}
\phi' \left(   Tr \left\{  \boldsymbol{\Sigma}^{-1} \mathbf{Z}_k \right\} \right)    .
\\
\end{aligned}
\end{equation} 
In order to compute the expectations, we recall that $ \mathbf{Z}_k = \mathbf{z}_k \mathbf{z}_k^H$ and that $\mathbf{z}_k$ has the stochastic representation $\mathbf{z}_k \overset{d}{=}   \sqrt{\mathcal{Q}}_k ~\boldsymbol{\Sigma}^{1/2} ~\mathbf{u}_k$.
This allows us some simplifications since
$ {\rm Tr} \left\{ \boldsymbol{\Sigma}^{-1} \mathbf{Z}_k   \right\} =  \mathcal{Q}_k $, $\mathbf{u}_k^H \mathbf{u}_k = 1$, and since that $\mathbf{u}_k$ and $\mathcal{Q}_k$ are independent (allowing to split the expectations).
Hence we have for the first term:
\begin{equation}
\label{eq:proof_first_expectation}
\footnotesize
\begin{aligned}
&
\mathbb{E}  \left[ {\rm Tr} \left\{ \left(      \boldsymbol{\Omega} \boldsymbol{\Sigma}^{-1} \right)^2  \mathbf{Z}_k \boldsymbol{\Sigma}^{-1} \right\}    \phi \left( {\rm Tr} \left\{  \boldsymbol{\Sigma}^{-1} \mathbf{Z}_k  \right\} \right) \right]  
\\
& = 
\mathbb{E}  \left[  {\rm Tr} \left\{   \boldsymbol{\Sigma}^{H/2} \boldsymbol{\Sigma}^{-1}  \left(     \boldsymbol{\Omega} \boldsymbol{\Sigma}^{-1} \right)^2   \boldsymbol{\Sigma}^{1/2} \mathbf{u}_k  \mathbf{u}^H_k  \right\}    \right]
\mathbb{E}  \left[ \mathcal{Q}_k  \phi \left(  \mathcal{Q}_k   \right) \right]
\\
& = - {\rm Tr} \left\{   \left( \boldsymbol{\Omega} \boldsymbol{\Sigma}^{-1} \right)^2 \right\}  
,
\end{aligned}
\end{equation}
where we used $\mathbb{E}\left[  \mathbf{u}_k\mathbf{u}_k^H \right]  = \mathbf{I}_M/M$ (since $\mathbf{u}_k \sim \mathcal{U}(\mathbb{C}\mathcal{S}^M)$), and \eqref{eq:pdf_2modular_variate} to obtain the result
\begin{equation}
\label{eq:expectation_modular_phi}
\mathbb{E}  \left[ \mathcal{Q}_k  \phi \left(  \mathcal{Q}_k   \right) \right]
= - M
.
\end{equation}
The second expectation is obtained by the same method as
\begin{equation}
\label{eq:proof_second_expectation}
\footnotesize
\begin{aligned}
&
\mathbb{E} \left[    {\rm Tr}^2\left\{ \boldsymbol{\Sigma}^{-1}    \boldsymbol{\Omega}  \boldsymbol{\Sigma}^{-1} \mathbf{Z}_k \right\}
\phi' \left(   {\rm Tr} \left\{  \boldsymbol{\Sigma}^{-1} \mathbf{Z}_k \right\} \right)
\right] 
\\
& = 
\mathbb{E} \left[   \left( \mathbf{u}^H_k     \boldsymbol{\Sigma}^{-H/2}  \boldsymbol{\Omega}  \boldsymbol{\Sigma}^{-1/2}  \mathbf{u}_k   \right)^2 \right]
\mathbb{E} \left[ \mathcal{Q}_k^2 \phi' \left( \mathcal{Q}_k  \right) \right] 
\\
& = 
\frac{\mathbb{E} \left[ \mathcal{Q}_k^2 \phi' \left( \mathcal{Q}_k  \right) \right]  
}{M(M+1)} 
\left(
{\rm Tr}^2 \left\{   \boldsymbol{\Omega}  \boldsymbol{\Sigma}^{-1} \right\}
+
{\rm Tr} \left\{  \left( \boldsymbol{\Omega}  \boldsymbol{\Sigma}^{-1} \right)^2 \right\}
\right),
\end{aligned}
\end{equation}
where we used the relation from \cite{besson2013fisher}, giving 
\begin{equation}
\mathbb{E} \left[   \left( \mathbf{u}^H_k    \mathbf{B} \mathbf{u}_k   \right)^2 \right] =  \frac{ 
{\rm Tr} \left\{  \mathbf{B}^2 \right\}+
{\rm Tr}^2 \left\{  \mathbf{B} \right\}  }{{M(M+1)} } ,
\end{equation}
for an arbitrary constant matrix $\mathbf{B}$ and $ \mathbf{u}_k \sim \mathcal{U} \left( \mathbb{C}  S^M \right)$.
Eventually, 
by plugging \eqref{eq:proof_first_expectation} and \eqref{eq:proof_second_expectation} into \eqref{eq:proof_eq_thm3} and \eqref{eq:proof_taylor}, the Fisher Information Metric is given as:
\begin{equation}
 g^{fim}_{\boldsymbol{\Sigma}} \left(  \boldsymbol{\Omega}, \boldsymbol{\Omega} \right) =  
 K \alpha    {\rm Tr}\left\{ \left( \boldsymbol{\Sigma}^{-1} \boldsymbol{\Omega} \right)^2 \right\}  + K \beta    {\rm Tr}^2 \left\{     \boldsymbol{\Omega}  \mathbf{R}^{-1} \right\}
,
\end{equation}
with coefficients $\alpha$ and $\beta$ defined in \eqref{eq:coefficients_metric}.
%\begin{equation}
%\left\{
%\begin{aligned}
%&\alpha &=~&   \left( 1   -  \frac{\mathbb{E} \left[ \mathcal{Q}_k^2 \phi' \left( \mathcal{Q}_k  \right) \right]  
%}{M(M+1)}   \right)
% \\
%&\beta  &=~& - \frac{}{M(M+1)} \mathbb{E} \left[ \mathcal{Q}_k^2 \phi' \left( \mathcal{Q}_k  \right) \right]  
%\end{aligned}
%\right.
%~.
%\end{equation}
Notice that $\beta = \alpha - 1$. Also, some manipulations with $\phi'(t) = g''(t)/g(t) - \phi^2(t) $, \eqref{eq:pdf_2modular_variate} and \eqref{eq:expectation_modular_phi} allow to show that
\begin{equation}
M(M+1)   -    \mathbb{E} \left[ \mathcal{Q}_k^2 \phi' \left( \mathcal{Q}_k  \right) \right]  
=
 \mathbb{E} \left[ \mathcal{Q}_k^2 \phi^2 \left( \mathcal{Q}_k  \right) \right] 
 , 
\end{equation}
which is consistent with the coefficients obtained in the parametric case \cite{besson2013fisher}.
To obtain the metric we now use the polarization formula
\begin{equation}
\label{eq:polar_formula}
\begin{aligned}
& g^{fim}_{\boldsymbol{\Sigma}} \left(  \boldsymbol{\Omega}_1,  \boldsymbol{\Omega}_2\right)
& = ~ &
\frac{1}{4}
\left[
g^{fim}_{\boldsymbol{\Sigma}} \left(  \boldsymbol{\Omega}_1 + \boldsymbol{\Omega}_2
,
\boldsymbol{\Omega}_1 + \boldsymbol{\Omega}_2 \right) \right.
\\
& & &
\left. -
g^{fim}_{\boldsymbol{\Sigma}} \left(  \boldsymbol{\Omega}_1 - \boldsymbol{\Omega}_2
,
\boldsymbol{\Omega}_1 - \boldsymbol{\Omega}_2 \right) 
\right] ,
\end{aligned}
\end{equation} 
which, after some expansions and simplifications leads to the conclusion of the proof.

\subsection{Proof of Theorem~\ref{thm:distance_ces}}
\label{appendix:proof_dist}

First, the directional derivative of $g^{{ces}}_{\boldsymbol{\Sigma}}(\boldsymbol{\Omega}_1,\boldsymbol{\Omega}_2)$ in the direction $\boldsymbol{\Omega}_3$, where $\boldsymbol{\Sigma}\in\mathcal{S}^{++}_M$ and $\boldsymbol{\Omega}_1,\boldsymbol{\Omega}_2,\boldsymbol{\Omega}_3\in\mathcal{S}_M$ is
\begin{multline}
		\D g^{{ces}}_{\boldsymbol{\Sigma}}(\boldsymbol{\Omega}_1,\boldsymbol{\Omega}_2)[\boldsymbol{\Omega}_3] = g^{{ces}}_{\boldsymbol{\Sigma}}(\D\boldsymbol{\Omega}_1[\boldsymbol{\Omega}_3],\boldsymbol{\Omega}_2)\\ + g^{{ces}}_{\boldsymbol{\Sigma}}(\boldsymbol{\Omega}_1,\D\boldsymbol{\Omega}_2[\boldsymbol{\Omega}_3])\\ 
		- \beta\tr(\boldsymbol{\Sigma}^{-1}\boldsymbol{\Omega}_3\boldsymbol{\Sigma}^{-1}\boldsymbol{\Omega}_1)\tr(\boldsymbol{\Sigma}^{-1}\boldsymbol{\Omega}_2) \\ - \beta\tr(\boldsymbol{\Sigma}^{-1}\boldsymbol{\Omega}_1)\tr(\boldsymbol{\Sigma}^{-1}\boldsymbol{\Omega}_3\boldsymbol{\Sigma}^{-1}\boldsymbol{\Omega}_2) \\
		- \alpha\tr(\boldsymbol{\Sigma}^{-1}(\boldsymbol{\Omega}_3\boldsymbol{\Sigma}^{-1}\boldsymbol{\Omega}_1 + \boldsymbol{\Omega}_1\boldsymbol{\Sigma}^{-1}\boldsymbol{\Omega}_3)\boldsymbol{\Sigma}^{-1}\boldsymbol{\Omega}_2) .
\label{eq:Dmetric_CES}
\end{multline}
It then follows from the Koszul formula (equation (5.11) in~\cite{absil2009optimization}) that the Levi-Civita connection $\nabla$ of $\boldsymbol{\Omega}_2$ in the direction $\boldsymbol{\Omega}_1$ on $\mathcal{S}^{++}_M$ endowed with metric~\eqref{eq:metric_CES} which is defined for all $\boldsymbol{\Sigma}\in\mathcal{S}^{++}_M$
\begin{equation}
		\nabla_{\boldsymbol{\Omega}_1}\boldsymbol{\Omega}_2 = \D\boldsymbol{\Omega}_2[\boldsymbol{\Omega}_1] - \symm(\boldsymbol{\Omega}_2\boldsymbol{\Sigma}^{-1}\boldsymbol{\Omega}_1),
\label{eq:Levi_Civita}
\end{equation}
where $\symm(\cdot)$ is the operator that returns the symmetrical part of its argument.
The Levi-Civita connection is the same as for the classical Riemannian metric in our case and we therefore have the same geodesics, which can be found for example in~\cite{bhatia2009positive}.
They can be characterized in two different (but equivalent) manners: the geodesics $\gamma$ on $\mathcal{S}^{++}_M$ are defined for all $\Sig\in\mathcal{S}^{++}_M$ and $\Omeg\in\mathcal{S}_M$ as
\begin{equation}
	\gamma(t) = \boldsymbol{\Sigma}^{\frac{1}{2}}\exp(t\boldsymbol{\Sigma}^{\frac{-1}{2}}\boldsymbol{\Omega}\boldsymbol{\Sigma}^{\frac{-1}{2}})\boldsymbol{\Sigma}^{\frac{1}{2}},
\end{equation}
where $\exp(\cdot)$ denotes the matrix exponential.
Equivalently, we can define the geodesic $\gamma$ between $\boldsymbol{\Sigma}_1$ and $\boldsymbol{\Sigma}_2$ in $\mathcal{S}^{++}_M$ as
\begin{equation}
	\gamma(t) = \boldsymbol{\Sigma}_1^{\frac{1}{2}}(\boldsymbol{\Sigma}_1^{\frac{-1}{2}}\boldsymbol{\Sigma}_2\boldsymbol{\Sigma}_1^{\frac{-1}{2}})^t\boldsymbol{\Sigma}_1^{\frac{1}{2}},
\end{equation} 
where $(\cdot)^t=\exp(t\log(\cdot))$ denotes the matrix power function defined through the matrix exponential and logarithm.
Furthermore, one can check that the metric~\eqref{eq:metric_CES} is invariant by congruence, \emph{i.e.}
\begin{equation}
	g^{{ces}}_{\U\boldsymbol{\Sigma}\U^T}(\U\boldsymbol{\Omega}_1\U^T,\U\boldsymbol{\Omega}_2\U^T) = g^{{ces}}_{\boldsymbol{\Sigma}}(\boldsymbol{\Omega}_1,\boldsymbol{\Omega}_2),
\end{equation}
for all $\boldsymbol{\Sigma}\in\mathcal{S}^{++}_M$, $\boldsymbol{\Omega}_1,\boldsymbol{\Omega}_2\in\mathcal{S}_M$ and invertible matrix $\U$.
Since we have the same geodesic and the congruence invariance property, the proof is completed by using the same steps given in~\cite{lang2012fundamentals} for the proof of the Riemannian distance on $\mathcal{S}^{++}_M$ equipped with the classical Riemannian metric ($\alpha=0$ and $\beta=1$).
